# Supplementary material for: Hydrogen Bond Strength Dictates the Rate-Limiting Steps of Diffusion in Proton-Conducting Perovskites:A Critical Length Perspective
Source: arXiv:2503.07291 source file (2026-07-18)
Supplement: Supplementary file 1 [file SupplementalMaterial.pdf]

**Supplemental Material for “Hydrogen Bond Strength Dictates the Rate-Limiting Steps of Diffusion in Proton-Conducting Perovskites: A Critical Length Perspective”**

Hang Ma, Ying Liang, Tianxing Ma<sup>\*</sup>, Jiajun Linghu<sup>\*</sup>, Zhipeng Li<sup>\*</sup>

School of Physics and Astronomy, Beijing Normal University, Beijing 100875, China

Key Laboratory of Multiscale Spin Physics (Ministry of Education), Beijing Normal University, Beijing 100875, China

Frontier Science Center for Flexible Electronics, Xi'an Institute of Flexible Electronics, Northwestern Polytechnical University, 127 Youyi West Road, Xi'an, Shaanxi, 710072, P.R. China Road, Xi'an, Shaanxi, 710072, P.R. China

<sup>\*</sup>Email:txma@bnu.edu.cn

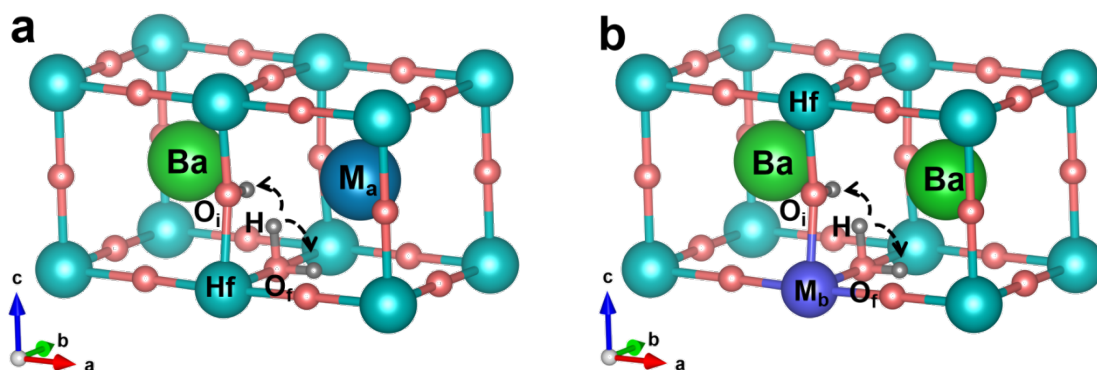

Fig.S1 a. Calculated rotation and transfer processes for A-site doped ( $M_a$ )  $BaHfO_3$  b. Calculated rotation and transfer processes for B-site doped ( $M_b$ )  $BaHfO_3$  .

Fig.S1 displays the calculated rotation and transfer processes for A-site ( $M_a$ ) and B-site doped ( $M_b$ )  $BaHfO_3$ . The doping concentrations of A-site ( $M_a = Sr^{2+}, K^+, Rb^+, Cs^+$ ) and B-site ( $M_b = Mg^{2+}, Ga^{3+}, In^{3+}, Sc^{3+}, Y^{3+}$ ) are 0.125, based on a  $2 \times 2 \times 2$  supercell. For the A-site doping system, we computed energy barrier of the proton rotation process around the A-site dopant ion (Fig. A1a), as well as the process of intra-octahedral proton transfer in the unit cell containing the A-site dopant ion (Fig. S1a, proton transfer from  $O_i$  to  $O_f$ ). For the B-site doping system, we computed energy barrier of the intra-octahedral proton transfer process around the B-site dopant ion (Fig. A1b, proton transfer from  $O_i$  to  $O_f$ ), as well as the proton rotation process at a specific oxygen site within the octahedron of the B-site dopant ion (Fig. S1b). These calculations are performed to investigate the impact of A-site and B-site doping on the proton rotation and transfer.

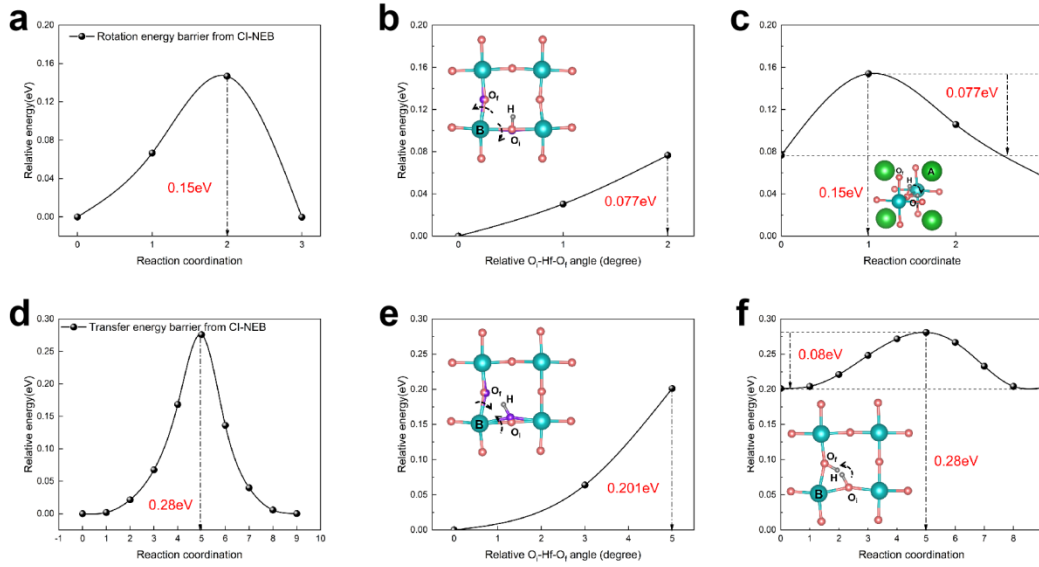

Fig.S2. the energy barriers for the elementary steps underlying proton rotation and transfer in the BaHfO<sub>3</sub>. a. the rotation energy barrier obtained from CI-NEB calculation. b. the energy barriers for the outward O<sub>i</sub>-B-O<sub>f</sub> bending motion during the proton rotation. c. the energy barriers for the hydroxide ion reorientation during the proton rotation. d. the transfer energy barrier obtained from CI-NEB calculation. e. the energy barriers for the inward O<sub>i</sub>-B-O<sub>f</sub> bending motion during the proton transfer. f. the energy barriers for the proton jumping during the proton transfer.

We calculated the energy barriers for the elementary steps underlying the rotation and transfer processes in undoped, A-site doped and B-site doped BaHfO<sub>3</sub> systems using density functional theory. For proton rotation, we calculated the energy barriers of outward O<sub>i</sub>-B-O<sub>f</sub> bending motion and hydroxide ion reorientation. For proton transfer, we calculated the energy barriers of inward O<sub>i</sub>-B-O<sub>f</sub> bending motion and proton jumping. By identifying a series of intermediate-angle structures (including saddle state) from the initial state to the saddle state, while fixing the positions of the moving ions O<sub>i</sub>, B and O<sub>f</sub>, we performed structure optimization for each intermediate-angle structure, and the position of proton also should be relaxed. The relative energy of the O<sub>i</sub>-B-O<sub>f</sub> bending motion can be obtained. When the O<sub>i</sub>-B-O<sub>f</sub> angle is same to the angle of the saddle state, fixing the O<sub>i</sub>-B-O<sub>f</sub> angle, the energy barriers of proton rotation and transfer is calculated by CI-NEB, which obtained the energy barrier for the hydroxide reorientation or the proton jumping.

Fig. S2 shows the comparison between the calculated energy barriers using CI-NEB and the energy barriers based on the elementary steps underlying rotation and transition for the BaHfO<sub>3</sub> system. During the proton rotation, the energy barriers for the outward O<sub>i</sub>-B-O<sub>f</sub> bending motion and the hydroxide ion reorientation are 0.077 eV (Fig. S2b) and 0.077 eV (Fig. S2c), respectively. Therefore, the total energy barrier based on these two elementary steps is 0.15 eV, which is consistent with the value of 0.15 eV obtained from our CI-NEB calculations(Fig. S2a). During the proton transfer, the energy barriers for the inward O<sub>i</sub>-B-O<sub>f</sub> bending motion and the proton jumping are calculated to be 0.20 eV and 0.08 eV, respectively. The total energy barrier based on these two elementary steps is 0.28 eV, which is also consistent with the CI-NEB calculation result of 0.28 eV (Fig. S2d). These results

confirm the validity of the proton rotation and transfer mechanism based on these elementary steps.

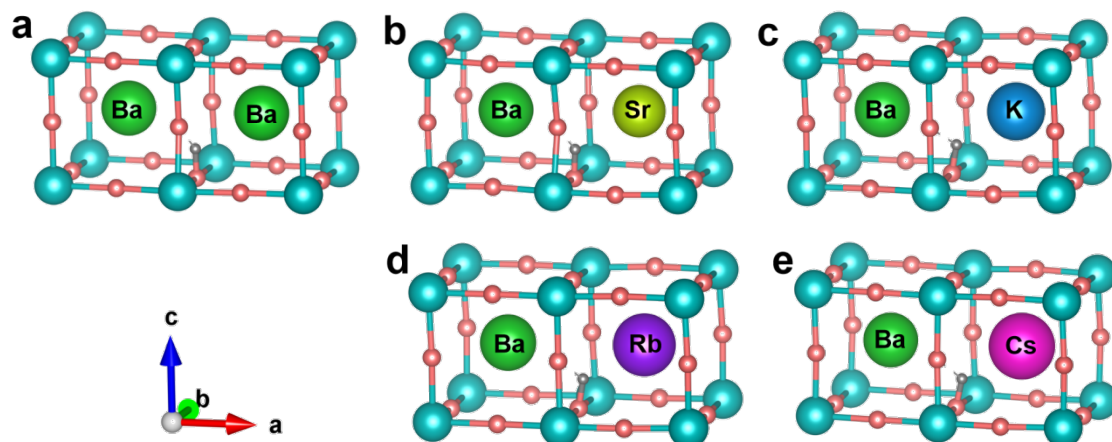

Fig.S3. illustrative diagram of the proton orientation in the BaHfO<sub>3</sub> and different A-site doped systems. a. undoped, b. Sr-doped, c. K-doped, d. Rb-doped, e. Cs-doped.

Fig.S3 displays the illustrative diagram of the proton orientation in the BaHfO<sub>3</sub> and different A-site doped systems. For systems doped with monovalent dopant ions such as K<sup>+</sup>, Rb<sup>+</sup>, and Cs<sup>+</sup>, the proton tilts towards the unit cell space occupied by the A-site dopant ions due to the net attractive force, as shown in Fig. S3c-e, resulting in the formation of relatively long hydrogen bonds (Table.1). Furthermore, due to the larger ionic radii of K<sup>+</sup>, Rb<sup>+</sup>, and Cs<sup>+</sup> (Ba<sup>2+</sup> = 1.61 Å, K<sup>+</sup> = 1.64 Å, Rb<sup>+</sup> = 1.72 Å, Cs<sup>+</sup> = 1.88 Å), the lattice of the unit cell expands, which also leads to an increase in hydrogen bond length. In previous studies, we found that as the ionic radius of the A-site dopant increases, the average M<sub>a</sub>-O bond length in the corresponding unit cell also increases, indicating a more pronounced lattice expansion effect. Consequently, the strength of the hydrogen bonds formed in the system decreases progressively in the order of K<sup>+</sup>, Rb<sup>+</sup>, and Cs<sup>+</sup> doping (Table 1). For systems doped with the divalent ion Sr<sup>2+</sup>, the unit cell contracted due to the smaller ionic radius of Sr<sup>2+</sup> (Fig. S3b). This effect shortens the hydrogen bond length formed between the proton and the acceptor oxygen ion theoretically.

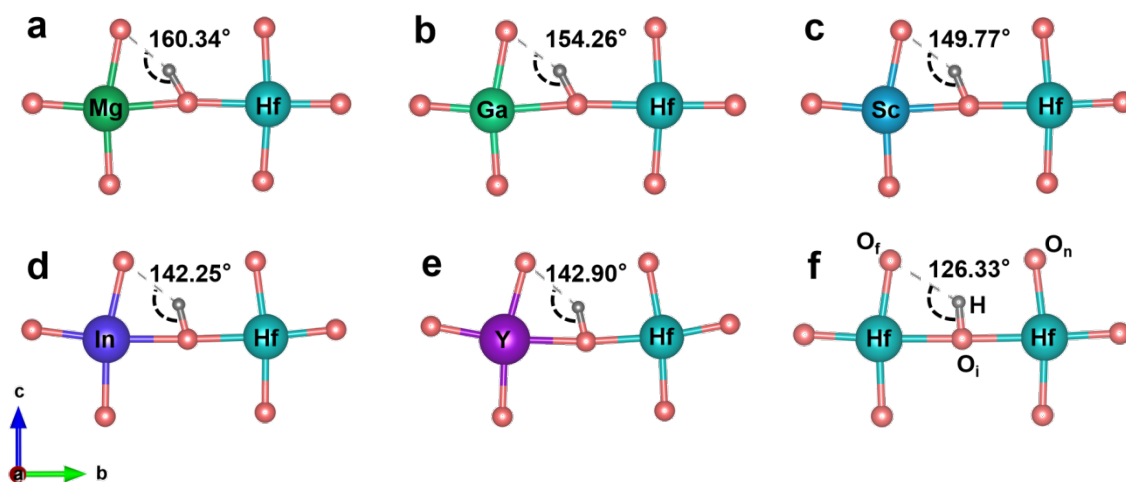

Fig.S4. illustrative diagram of the net attractive force on the proton exerted by B-site doped

ions. a. Mg-doped b. Ga-doped, c. Sc-doped, d. In-doped, e. Y-doped, f. undoped

|    | <b>Ionic radius(Å)</b> | <b>The average of M<sub>b</sub>-O(Å)</b> |
|----|------------------------|------------------------------------------|
| Ga | 0.62                   | 2.09                                     |
| Hf | 0.71                   | 2.10                                     |
| Mg | 0.72                   | 2.13                                     |
| Sc | 0.75                   | 2.13                                     |
| In | 0.8                    | 2.17                                     |
| Y  | 0.9                    | 2.22                                     |

Table.S1 Ionic radii of different B-site dopant ions and the corresponding octahedral unit cell parameters

Fig.S4 shows the illustrative diagram of the net attractive force on the proton exerted by B-site doped ions. Since  $Mg^{2+}$  has the lowest valence, it exerts the strongest net attractive force on the proton, resulting in the proton tilting to the greatest extent and the  $O_i-H...O_f$  hydrogen bond approaching the most linear configuration (close to  $180^\circ$ ) (Fig. S4a), which the formed hydrogen bond  $H...O_f$  is the shortest (Table.1). For the trivalent dopant ions  $Ga^{3+}$ ,  $Sc^{3+}$ ,  $In^{3+}$ , and  $Y^{3+}$ , it can be observed that as the ionic radius increases, the formed hydrogen bonds weaken (Table 1). This is because a larger ionic radius such as  $In^{3+}$  and  $Y^{3+}$  leads to the expansion of the surrounding octahedron (Table.S1. By measuring the average distance between the B-site dopant ion and the six coordinated oxygen ions. ), which shortens the distance between the proton and the oxygen ion  $O_n$  in the adjacent octahedron, promoting the formation of the hydrogen bond  $H...O_n$ . However, the attraction between the proton and the oxygen ion  $O_n$  in the adjacent octahedron weakens the net attractive force of the B-site dopant ions on the proton, thus reducing the tilt of the proton. As a result, the degree of  $\angle O_iHO_f$  decreases (Fig.S4d,e), leading to a longer hydrogen bond length (Table.1)<sup>[1][2]</sup>.

|                                    | <b>Initial BaHfO<sub>3</sub> system</b> | <b>BaHfO<sub>3</sub> system after 5% compression</b> | <b>BaHfO<sub>3</sub> system after 5% compression in the xy direction</b> | <b>BaHfO<sub>3</sub> system after 1% stretching</b> |
|------------------------------------|-----------------------------------------|------------------------------------------------------|--------------------------------------------------------------------------|-----------------------------------------------------|
| <b>H...O<sub>f</sub></b>           | 2.15 Å                                  | 2.04 Å                                               | 2.07 Å                                                                   | 2.17 Å                                              |
| <b>Δ<sub>energy barriers</sub></b> | -0.13 eV                                | 0.08 eV                                              | 0 eV                                                                     | -0.16 eV                                            |

Table.S2 The hydrogen bond lengths and energy barrier differences for rotation and transfer  $\Delta_{\text{energy barriers}}$  ( $\Delta_{\text{energy barriers}} = E_{\text{rotation}} - E_{\text{transfer}}$ ) in the initial BaHfO<sub>3</sub> system and after 5% compression and 1% stretching.

The purpose of Table S2 is to verify that the strength of hydrogen bonds is the main factor influencing the energy barrier differences for rotation and transfer. In the initial BaHfO<sub>3</sub> system, the hydrogen bond length  $H...O_f$  is 2.15 Å, with the rotation energy barrier being 0.13 eV lower than the transfer energy barrier; After 1% stretching, the rotation energy barrier is the lowest, 0.16 eV smaller than the transfer energy barrier; Through 5% compression, the

hydrogen bond strengthens, with the length reducing to 2.04 Å, and the rotation energy barrier becomes 0.08 eV higher than the transfer energy barrier; By 5% compression along the xy direction to alter the cubic structure of BaHfO<sub>3</sub>, The hydrogen bond length decreases to 2.07 Å, at which point the rotation energy barrier equals the transfer. In addition, we also calculated SrCeO<sub>3</sub> which are more closely packed and strongly deviate from the cubic perovskite structure. The length of hydrogen bond is 1.71 Å, and the  $\Delta_{\text{energy barriers}}$  is 0.13 eV.

As the hydrogen bond length weakens, it can be observed that the difference between the rotation and transfer energy barriers changes from positive to negative. This large negative difference directly leads to more than one order of magnitude disparity in the residence times of the two processes. Therefore, this demonstrates that the strength of the hydrogen bond is a crucial factor in determining whether the transfer process is rate-limiting.

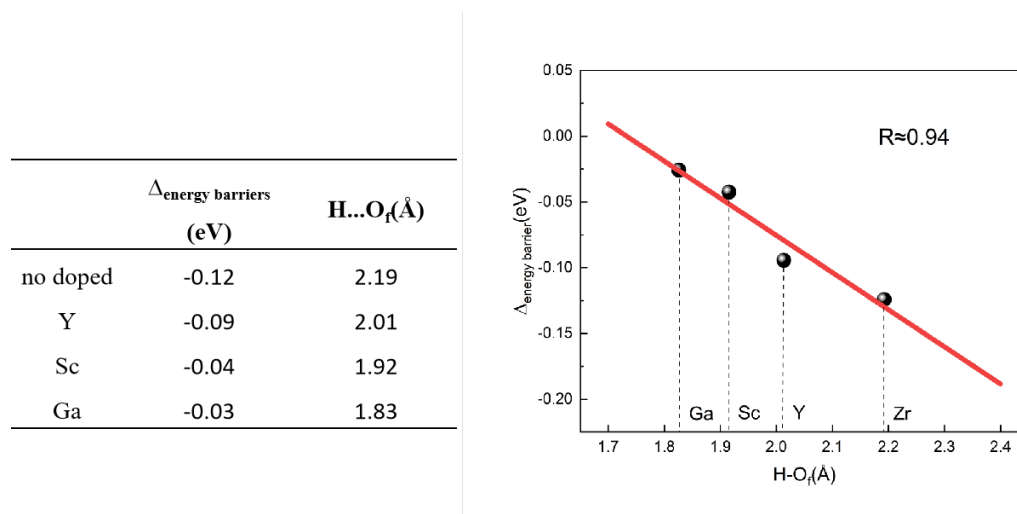

Fig.S5. The left table is energy barrier differences for rotation and transfer  $\Delta_{\text{energy barriers}}$  as well as the hydrogen bond length H...O<sub>f</sub> in the BaZrO<sub>3</sub> system, B-site doped( $M_b = \text{Ga}^{3+}, \text{Sc}^{3+}, \text{Y}^{3+}$ ) systems. The right figure shows the linear fitting results of the data in the table. (The black dots represent the original data points, and the red solid line represents the linear fitting curve.)

Since the critical hydrogen bond value determining the rate-limiting step of proton transfer in the article was obtained through fitting for the BaHfO<sub>3</sub> system, we calculated the common proton-conducting perovskite BaZrO<sub>3</sub> and its typical doped systems to verify the existence of this critical hydrogen bond and the universality of its value. From Equation (1), we can deduce that the energy barrier difference between rotation and transfer processes corresponding to the critical hydrogen bond is approximately in the range of -0.15 eV to -0.1 eV. Therefore, from the fitted plot in Fig. S5, we can observe that the critical hydrogen bond in the pure BaZrO<sub>3</sub> system is around 2.19Å, which is close to the critical hydrogen bond value of 2.08Å~2.16 Å reported in our article. Additionally, both pure systems fall within the range of the critical hydrogen bond. Through B-site doping, the hydrogen bond strengthens, the energy barrier difference decreases, and proton transfer can no longer be considered the rate-limiting step. This implies that for stable cubic structures like BaZrO<sub>3</sub> and BaHfO<sub>3</sub>, the rotation process should not be neglected when studying proton conduction phenomena in B-

site doped systems.

Additionally, from the fitted plot in Fig. S5, it can be seen that the coefficient of determination  $R$  for the linear fit is approximately 0.94, which is the highest among all higher-order fits. Therefore, as the hydrogen bond strength decreases, the energy barrier difference between rotation and transfer increases, further confirming that hydrogen bonding is the determining factor for the rotation-transfer energy barrier difference.

#### References:

1. Björketun M E, Sundell P G, Wahnström G. Effect of acceptor dopants on the proton mobility in Ba Zr O 3: A density functional investigation[J]. Physical Review B—Condensed Matter and Materials Physics, 2007, 76(5): 054307.
2. Bévillon É, Hermet J, Dezanneau G, et al. How dopant size influences the protonic energy landscape in BaSn  $1-x$  M  $x$  O  $3-x/2$  (M= Ga, Sc, In, Y, Gd, La)[J]. Journal of Materials Chemistry A, 2014, 2(2): 460-471.
